# Supplementary material for: Developing Theoretical Foundations for Runtime Enforcement
Source: arXiv:1804.08917 source file (2018-11-12)
Supplement: Supplementary file 1 [file rel-enf-mon-proofs.tex]

In this section we present the proofs related to establishing a relation between enforceability and monitorability.

\subsection{Proving Correspondence between the Original and Alternative Definitions for Monitorability}
\label{sec:app:rel-mon-amon-proof}

\newcommand{\pSat}{\pV\vSat\hV} %% Logic Notation
\newcommand{\pVio}{\pV\nvSat\hV}

\noindent We now need to prove that
$$ \forall\hV\in\uhml,m\in\Mon\cdot\amondef{m}{\hV}\Leftrightarrow\mondef{m}{\hV} $$
We therefore prove the following:
\begin{enumerate}[\qquad$(a)$]
	\item $\forall\hV\in\uhml,m\in\Mon\cdot\mondef{m}{\hV}\Rightarrow\amondef{m}{\hV}$ \label{rtp:mon-to-amon}
	\item $\forall\hV\in\uhml,m\in\Mon\cdot\amondef{m}{\hV}\Rightarrow\mondef{m}{\hV}$ \label{rtp:amon-to-mon}
\end{enumerate}

\begin{proof}[ for (a)]  We initially know 
	\begin{gather}
		\mondef{m}{\hV} \label{proof-mon-to-amon-1}
	\end{gather}
	By \pref{proof-mon-to-amon-1} and defn of \mondef{m}{\hV} we know 
	\begin{gather}
		\smondef{m}{\hV} \label{proof-mon-to-amon-2} \\
		\cmondef{m}{\hV} \label{proof-mon-to-amon-3}
	\end{gather}
	By \pref{proof-mon-to-amon-2} and defn of \smondef{m}{\hV} we know 
	\begin{gather}
		\forall \pV\cdot\monacc{\pV}{m}\imp \pSat \label{proof-mon-to-amon-4} \\
		\forall \pV\cdot\monrej{\pV}{m}\imp \pVio \label{proof-mon-to-amon-5}
	\end{gather}
	In \cite{Francalanza2015Mon}, Francalanza \etal prove \emph{Theorem 2} (stated below), which states that multi-verdict monitors are not monitorable \wrt their defn of monitorability (\ie \mondef{\mV}{\hV}).
	\\[2mm]\textbf{Theorem 2 (Multi-verdict Monitors)} For all monitors $\mV\in\Mon$.
	\begin{center}
		$(\exists t,u\in\Act*\cdot \mV\wtraS{t}\myes \text{ and } \mV\wtraS{t}\mno) \imp \nexists\hV\in\uhml\cdot\mondef{\mV}{\hV}$
	\end{center}		
	Hence, we also know that sound monitors (denoted by \textsf{smon}) are \emph{univerdict}. This means that a monitor may either reject or accept a program \emph{but not both}.
	%By \pref{proof-mon-to-amon-2} and Francalanza \etal's Theorem 2 in \cite{Francalanza2015Mon} we also know that sound monitors (denoted by \textsf{smon}) are \emph{univerdict}. This means that a monitor may either reject or accept a program \emph{but not both}. Hence we know
	\begin{gather}
		\forall \pV,\nexists m\in\Mon\cdot\monacc{\pV}{m} \text{   and   } \monrej{\pV}{m} \label{proof-mon-to-amon-6} 
	\end{gather}
	By \pref{proof-mon-to-amon-3} and defn of \cmondef{m}{\hV} we know 
	\begin{gather}
		\scmondef{m}{\hV} \text{  or  }	\vcmondef{m}{\hV} \label{proof-mon-to-amon-7}
	\end{gather}
	By \pref{proof-mon-to-amon-7} and defn of \scmondef{m}{\hV} and \vcmondef{m}{\hV}  we know 
	\begin{gather}
		(\forall \pV\cdot \pSat \imp \monacc{\pV}{m}) \text{  or  }	(\forall \pV\cdot \pVio \imp \monrej{\pV}{m}) \label{proof-mon-to-amon-8}
	\end{gather}
	We consider the following cases separately:
	
	\begin{case-noreset}[\pSat]
		Since $\pSat$, from \pref{proof-mon-to-amon-8} we know that there cannot exist a monitor which rejects any program $\pV$ as this would require that $\pVio$ (which is the negation of what we know \ie that $\pSat$). Moreover, since we know that $\pSat$, from \pref{proof-mon-to-amon-8} we can conclude
		\begin{gather}
			\forall \pV\cdot \pSat \imp \monacc{\pV}{m} \label{proof-mon-to-amon-9}
		\end{gather}
		Since $\pSat$, from \pref{proof-mon-to-amon-9} we can deduce
		\begin{gather}
			\monacc{\pV}{m} \label{proof-mon-to-amon-10}
		\end{gather}
		By \pref{proof-mon-to-amon-6} and \pref{proof-mon-to-amon-10} we know that the premise of \pref{proof-mon-to-amon-5} cannot be true, meaning that \pref{proof-mon-to-amon-5} is trivially satisfied. On the other hand, we know that \pref{proof-mon-to-amon-4} holds because of \pref{proof-mon-to-amon-10}. Hence, by \pref{proof-mon-to-amon-4} and \pref{proof-mon-to-amon-9} we can conclude
		\begin{gather}
				(\forall \pV\cdot \pSat \imp \monacc{\pV}{m}) \text{  and  } (\forall \pV\cdot\monacc{\pV}{m}\imp \pSat) \label{proof-mon-to-amon-11}
		\end{gather}
		By \pref{proof-mon-to-amon-11} and the defn of \textsf{pmon} we know
		\begin{gather}
			\pmondef{m}{\hV} \label{proof-mon-to-amon-12}
		\end{gather}		
	\end{case-noreset}
	\begin{case-noreset}[\pVio]
		Using a very similar argument as in the previous case, we can conclude
		\begin{gather}
			\nmondef{m}{\hV} \label{proof-mon-to-amon-13}
		\end{gather}
	\end{case-noreset}
	\noindent Hence, since $\pSat$ is the complement of $\pVio$ we can conclude that for our univerdict (sound) monitors (as shown by \pref{proof-mon-to-amon-6}), either \pref{proof-mon-to-amon-12} or \pref{proof-mon-to-amon-13} can be true but \emph{not both}. Hence, we can conclude
	\begin{gather}
		\pmondef{m}{\hV} \text{   or   }\nmondef{m}{\hV} \label{proof-mon-to-amon-14}
	\end{gather}
	By \pref{proof-mon-to-amon-14} and defn of \textsf{amon} we know
	\begin{gather*}
		\amondef{m}{\hV} 
	\end{gather*}
\end{proof}\bigskip\bigskip

\begin{proof}[ for (b)] We initially know 
	\begin{gather}
		\amondef{m}{\hV} \label{proof-amon-to-mon-1}
	\end{gather}
	By \pref{proof-amon-to-mon-1} and defn of \amondef{m}{\hV} we know 
	\begin{gather}
		\nmondef{m}{\hV} \text{  or  } \pmondef{m}{\hV} \label{proof-amon-to-mon-2}
	\end{gather}
	We individually consider the possibilities for satisfying \pref{proof-amon-to-mon-2}:
	
	\begin{case}[\text{\textsf{pmon} is \textsl{true} while \textsf{nmon} is \textsl{false}}]
		By the case hypothesis we know
		\begin{gather}
			\nmondef{m}{\hV} \text{ is \emph{true}} \label{proof-amon-to-mon-3}\\
			\pmondef{m}{\hV} \text{ is \emph{false}} \label{proof-amon-to-mon-4}
		\end{gather}
		By \pref{proof-amon-to-mon-3} and defn of \textsf{pmon} we know
		\begin{gather}
			\forall \pV\cdot\monacc{\pV}{m}\imp \pSat (\,=\,\emph{true}) \label{proof-amon-to-mon-5}\\
			\forall \pV\cdot \pSat\imp\monacc{\pV}{m} (\,=\,\emph{true}) \label{proof-amon-to-mon-6}
		\end{gather}
		By \pref{proof-amon-to-mon-4} and defn of \textsf{nmon} we know
		\begin{gather}
			\forall \pV\cdot\monrej{\pV}{m}\imp \pVio (\,=\,\emph{false}) \label{proof-amon-to-mon-7}\\
			\forall \pV\cdot \pVio\imp\monrej{\pV}{m} (\,=\,\emph{false}) \label{proof-amon-to-mon-8}
		\end{gather}
		Since \pref{proof-amon-to-mon-6} is \emph{true}, we know that $\pV\!\in\!\syn{\hV}$, however since \pref{proof-amon-to-mon-8} is \emph{false} this means that $\pV\!\notin\!\syn{\hV}$ as otherwise the entire implication (\ie \pref{proof-amon-to-mon-8}) would resolve to \emph{true}. Hence, this case is satisfied trivially since \pref{proof-amon-to-mon-6} and \pref{proof-amon-to-mon-8} \emph{contradict} each other.		
	\end{case}
	
	\begin{case}[\text{\textsf{pmon} is \textsl{false} while \textsf{nmon} is \textsl{true}}] The proof for this case is very similar to that for the other cases.
	\end{case}
	
	\begin{case}[\text{Both \textsf{pmon} and \textsf{nmon} are \textsl{true}}]
		By the case hypothesis we know
		\begin{gather}
			\nmondef{m}{\hV} \text{ is \emph{true}} \label{proof-amon-to-mon-9}\\
			\pmondef{m}{\hV} \text{ is \emph{true}} \label{proof-amon-to-mon-10}
		\end{gather}
		By \pref{proof-amon-to-mon-9} and defn of \textsf{pmon} we know
		\begin{gather}
			\forall \pV\cdot\monacc{\pV}{m}\imp \pSat (\,=\,\emph{true}) \label{proof-amon-to-mon-11}\\
			\forall \pV\cdot \pSat\imp\monacc{\pV}{m} (\,=\,\emph{true}) \label{proof-amon-to-mon-12}
		\end{gather}
		By \pref{proof-amon-to-mon-10} and defn of \textsf{nmon} we know
		\begin{gather}
			\forall \pV\cdot\monrej{\pV}{m}\imp \pVio (\,=\,\emph{true}) \label{proof-amon-to-mon-13}\\
			\forall \pV\cdot \pVio\imp\monrej{\pV}{m} (\,=\,\emph{true}) \label{proof-amon-to-mon-14}
		\end{gather}
		Hence, by \pref{proof-amon-to-mon-11}, \pref{proof-amon-to-mon-13} and defn of \textsf{smon} we know
		\begin{gather}
			\smondef{m}{\hV} \label{proof-amon-to-mon-15}
		\end{gather}
		By introducing a disjunction on \pref{proof-amon-to-mon-12} and \pref{proof-amon-to-mon-14}, we know
		\begin{gather}
			(\pSat \imp \monacc{\pV}{m}) \text{  or  } (\pVio \imp \monrej{\pV}{m}) \label{proof-amon-to-mon-16}
		\end{gather}
		By \pref{proof-amon-to-mon-16} and defn of \textsf{cmon} we know
		\begin{gather}
			\cmondef{m}{\hV} \label{proof-amon-to-mon-17}
		\end{gather}
		By \pref{proof-amon-to-mon-15}, \pref{proof-amon-to-mon-17} and defn of \textsf{mon} we know
		\begin{gather}
			\mondef{m}{\hV} \label{proof-amon-to-mon-18}
		\end{gather}
	\end{case}	
\end{proof}

\subsection{Proving the Relationship between Strong Enforceability and Negative Monitorability}
\label{sec:app:rel-mon-enf-proof}
\begin{rtp}
	$\forall\hV\in\uhml\cdot\, \enfmonrel{\g{\hV}{\rho}}{\gRV{\hV}}$\\[2mm]
	To Prove this theorem we must show that relation \R (below) \emphbf{relates enforceability to monitorability}.
	$$\R \defEquals \big\{(\g{\hV}{\rho},\gRV{\hV})\;\vert\; \g{\hV}{\rho}=\eV \text{ and }\gRV{\hV}=\mV \big\}$$
\end{rtp}

\ic{I'M NOT ENTIRELY SURE WHETHER THIS PROOF MAKES ANY SENSE!!!!}

\begin{proof} By coinduction on the structure of $\hV$. 
	\\\begin{proofRemark}
		[Since \g{\hV} is defined exclusively for formulae that are expressible in \shmlwf, any other formula $\hV\in\uhml$ but $\hV\notin\shmlwf$ cannot be synthesised into an enforcement monitor and thus cause the premise of the theorem being proven to evaluate to false, thereby leading the theorem to be trivially satisfied. Hence, it suffices to conduct our coinductive proof \wrt $\hV\in\shmlwf$.\medskip]
	\end{proofRemark}\vspace{-5mm}

	\begin{case}[\hV=\htru] \ic{THIS CASE IS CAUSING TROUBLE!!}	\end{case} 
	
	\begin{case}[\hV=\hVarX] Does not apply since $\hVarX$ is an open formula. \end{case} 	

	\begin{case}[\hV=\hfls] 
		\newcommand{\formula}{\hfls}
		Initially we know
		\begin{gather}
			\enfdef{\g{\formula}{\rho}}{\formula}\label{proof:enf-mon-rel-ff-1}
		\end{gather}
		Since $\hV=\formula$, by defn of \g{-} and \gRV{-} we know
		\begin{gather}
			\g{\formula}{\rho}=\mend \label{proof:enf-mon-rel-ff-2}\\
			\gRV{\formula}=\mno \label{proof:enf-mon-rel-ff-3}
		\end{gather}
		Since \formula cannot be satisfied by any process $\pV$, we can deduce
		\begin{gather}
			\forall \pV\cdot\, \pV\nvSat\formula \label{proof:enf-mon-rel-ff-4}
		\end{gather}
		Moreover, from \pref{proof:enf-mon-rel-ff-3} and the defn of \textsf{rej}, we know
		\begin{gather}
			\forall \pV\cdot\, \monrej{\pV}{\gRV{\formula}} \label{proof:enf-mon-rel-ff-5}
		\end{gather}
		By \pref{proof:enf-mon-rel-ff-4} and \pref{proof:enf-mon-rel-ff-5}, we can thus deduce
		\begin{gather}
			\forall \pV\cdot\, \pV\nvSat\formula\, \imp\, \monrej{\pV}{\gRV{\formula}} \label{proof:enf-mon-rel-ff-6}\\
			\forall \pV\cdot\, \monrej{\pV}{\gRV{\formula}}\, \imp\, \pV\nvSat\formula \label{proof:enf-mon-rel-ff-7}
		\end{gather}
		Finally, by \pref{proof:enf-mon-rel-ff-6}, \pref{proof:enf-mon-rel-ff-7} and the defn of \textsf{nmon} we know
		\begin{gather}
			\nmondef{\gRV{\formula}}{\formula}
		\end{gather}
	\end{case} 
		
	\begin{case}[\hV=\hmax{\hVarX}{\hV}]
		\newcommand{\formula}{\hmax{\hVarX}{\hV}}
		\newcommand{\subform}{\hV\sub{\formula}{\hVarX}}
		\newcommand{\recsubenf}{\g{\hV}{\rho}\sub{\mrec{\mx}{\g{\hV}{\rho}}}{\mx}}
		\newcommand{\recsubmon}{\gRV{\hV}{\rho}\sub{\mrec{\mx}{\gRV{\hV}{\rho}}}{\mx}}
		Initially we know
		\begin{gather}
			\enfdef{\g{\formula}{\rho}}{\formula}\label{proof:enf-mon-rel-max-1}
		\end{gather}
		Since $\formula\,\equiv\,\subform$, from \pref{proof:enf-mon-rel-max-1} we know
		\begin{gather}
			\enfdef{\g{\subform}{\rho}}{\subform}\label{proof:enf-mon-rel-max-2}
		\end{gather}
		Since $\hV=\formula$, by defn of \g{-} and \gRV{-} we know
		\begin{gather}
			\g{\formula}{\rho}=\recsubenf \label{proof:enf-mon-rel-max-3}\\
			\gRV{\formula}=\recsubmon \label{proof:enf-mon-rel-max-4}
		\end{gather}
		By \pref{proof:enf-mon-rel-max-3}, \pref{proof:enf-mon-rel-max-4} and defn of \R we know
		\begin{gather}
			(\recsubenf,\recsubmon)\in\R \label{proof:enf-mon-rel-max-5}
		\end{gather}
		By \pref{proof:enf-mon-rel-max-5} and IH we know
		\begin{gather}
			\enfdef{\recsubenf}{\subform} \imp \nmondef{\recsubmon}{\subform} \label{proof:enf-mon-rel-max-6}
		\end{gather}
		By \pref{proof:enf-mon-rel-max-3}, \pref{proof:enf-mon-rel-max-6} and since $\formula\,\equiv\,\subform$ we know
		\begin{gather}
			\enfdef{\g{\formula}{\rho}}{\formula} \imp \nmondef{\recsubmon}{\subform} \label{proof:enf-mon-rel-max-7}
		\end{gather}
		From \pref{proof:enf-mon-rel-max-1} and \pref{proof:enf-mon-rel-max-7} we deduce
		\begin{gather}
			\nmondef{\recsubmon}{\subform} \label{proof:enf-mon-rel-max-8}
		\end{gather}
		Finally, by \pref{proof:enf-mon-rel-max-3}, \pref{proof:enf-mon-rel-max-4}, \pref{proof:enf-mon-rel-max-8} and since $\formula\,\equiv\,\subform$ we conclude
		\begin{gather}
			\nmondef{\gRV{\formula}}{\formula}
		\end{gather}		
	\end{case} 	

	\begin{case}[\hV=\hAnd\hgnec{\pate_i}{c_i}\hV_i]
		\newcommand{\formula}{\hAnd\hgnec{\pate_i}{c_i}\hV_i}
		\newcommand{\subenf}{
			\begin{xbrackets}{c}
			\mCh
			\begin{xbrace}{ll}
				\mdropc{\pate_i}{c_i}{\g{\varphi_i}{\rho}} & \quad \text{if }\dc{{\varphi_i}}=\ctru\!\!\!\\
				\mact{\pate_i}{c_i}{\g{\varphi_i}{\rho}} & \quad \text{otherwise} \!\!\!
			\end{xbrace}
			\end{xbrackets}}
		\newcommand{\submon}{\mCh\mact{\pate_i}{c_i}{\gRV{\varphi_i}}}
		Initially we know
		\begin{gather}
		\enfdef{\g{\formula}{\rho}}{\formula}\label{proof:enf-mon-rel-nec-1}
		\end{gather}
		Since $\hV=\formula$, by defn of $\g{-}{\rho}$ and \gRV{-} we know
		\begin{gather}
			\g{\formula}{\rho}=\subenf \label{proof:enf-mon-rel-nec-2}\\
			\gRV{\formula}=\mCh\gRV{\hgnec{\pate_i}{c_i}{\varphi_i}}=\submon \label{proof:enf-mon-rel-nec-3}
		\end{gather}
		By \pref{proof:enf-mon-rel-nec-2}, \pref{proof:enf-mon-rel-nec-3} and defn of \R we know
		\begin{gather}
			(\subenf,\submon)\in\R \label{proof:enf-mon-rel-nec-4}
		\end{gather}
		By \pref{proof:enf-mon-rel-nec-4} and IH we know
		\begin{gather}
			\begin{array}{r}
				\enfdef{\subenf}{\formula} \\ \hfill\imp \nmondef{\submon}{\formula} 
			\end{array}\label{proof:enf-mon-rel-nec-5}
		\end{gather}
		From \pref{proof:enf-mon-rel-nec-1}, \pref{proof:enf-mon-rel-nec-2} and \pref{proof:enf-mon-rel-nec-5} we can deduce
		\begin{gather}
			\nmondef{\submon}{\formula} \label{proof:enf-mon-rel-nec-6}
		\end{gather}
		Finally, by \pref{proof:enf-mon-rel-nec-5} and \pref{proof:enf-mon-rel-max-6} we can conclude
		\begin{gather}
			\nmondef{\gRV{\formula}}{\formula}
		\end{gather}		
	\end{case}	
\end{proof}
%\ic{HOW SHOULD WE PROVE THIS!! Should we do it \wrt \shml?}
