# Supplementary material for: Developing Theoretical Foundations for Runtime Enforcement
Source: arXiv:1804.08917 source file (2018-11-12)
Supplement: Supplementary file 2 [file alt-mon-def-proof.tex]

\newcommand{\pSat}{\pV\vSat\hV} %% Logic Notation
\newcommand{\pVio}{\pV\nvSat\hV}

\noindent We now need to prove that
$$ \forall\hV\in\uhml,m\in\Mon\cdot\amondef{m}{\hV}\Leftrightarrow\mondef{m}{\hV} $$
We therefore prove the following:
\begin{enumerate}[\qquad$(a)$]
	\item $\forall\hV\in\uhml,m\in\Mon\cdot\mondef{m}{\hV}\Rightarrow\amondef{m}{\hV}$ \label{rtp:mon-to-amon}
	\item $\forall\hV\in\uhml,m\in\Mon\cdot\amondef{m}{\hV}\Rightarrow\mondef{m}{\hV}$ \label{rtp:amon-to-mon}
\end{enumerate}

\begin{proof}[ for (a)]  We initially know 
	\begin{gather}
		\mondef{m}{\hV} \label{proof-mon-to-amon-1}
	\end{gather}
	By \pref{proof-mon-to-amon-1} and defn of \mondef{m}{\hV} we know 
	\begin{gather}
		\smondef{m}{\hV} \label{proof-mon-to-amon-2} \\
		\cmondef{m}{\hV} \label{proof-mon-to-amon-3}
	\end{gather}
	By \pref{proof-mon-to-amon-2} and defn of \smondef{m}{\hV} we know 
	\begin{gather}
		\forall \pV\cdot\monacc{\pV}{m}\imp \pSat \label{proof-mon-to-amon-4} \\
		\forall \pV\cdot\monrej{\pV}{m}\imp \pVio \label{proof-mon-to-amon-5}
	\end{gather}
	In \cite{Francalanza2015Mon}, Francalanza \etal prove \emph{Theorem 2} (stated below), which states that multi-verdict monitors are not monitorable \wrt their defn of monitorability (\ie \mondef{\mV}{\hV}).
	\\[2mm]\textbf{Theorem 2 (Multi-verdict Monitors)} For all monitors $\mV\in\Mon$.
	\begin{center}
		$(\exists t,u\in\Act*\cdot \mV\wtraS{t}\myes \text{ and } \mV\wtraS{t}\mno) \imp \nexists\hV\in\uhml\cdot\mondef{\mV}{\hV}$
	\end{center}		
	Hence, we also know that sound monitors (denoted by \textsf{smon}) are \emph{univerdict}. This means that a monitor may either reject or accept a program \emph{but not both}.
	%By \pref{proof-mon-to-amon-2} and Francalanza \etal's Theorem 2 in \cite{Francalanza2015Mon} we also know that sound monitors (denoted by \textsf{smon}) are \emph{univerdict}. This means that a monitor may either reject or accept a program \emph{but not both}. Hence we know
	\begin{gather}
		\forall \pV,\nexists m\in\Mon\cdot\monacc{\pV}{m} \text{   and   } \monrej{\pV}{m} \label{proof-mon-to-amon-6} 
	\end{gather}
	By \pref{proof-mon-to-amon-3} and defn of \cmondef{m}{\hV} we know 
	\begin{gather}
		\scmondef{m}{\hV} \text{  or  }	\vcmondef{m}{\hV} \label{proof-mon-to-amon-7}
	\end{gather}
	By \pref{proof-mon-to-amon-7} and defn of \scmondef{m}{\hV} and \vcmondef{m}{\hV}  we know 
	\begin{gather}
		(\forall \pV\cdot \pSat \imp \monacc{\pV}{m}) \text{  or  }	(\forall \pV\cdot \pVio \imp \monrej{\pV}{m}) \label{proof-mon-to-amon-8}
	\end{gather}
	We consider the following cases separately:
	
	\begin{case-noreset}[\pSat]
		Since $\pSat$, from \pref{proof-mon-to-amon-8} we know that there cannot exist a monitor which rejects any program $\pV$ as this would require that $\pVio$ (which is the negation of what we know \ie that $\pSat$). Moreover, since we know that $\pSat$, from \pref{proof-mon-to-amon-8} we can conclude
		\begin{gather}
			\forall \pV\cdot \pSat \imp \monacc{\pV}{m} \label{proof-mon-to-amon-9}
		\end{gather}
		Since $\pSat$, from \pref{proof-mon-to-amon-9} we can deduce
		\begin{gather}
			\monacc{\pV}{m} \label{proof-mon-to-amon-10}
		\end{gather}
		By \pref{proof-mon-to-amon-6} and \pref{proof-mon-to-amon-10} we know that the premise of \pref{proof-mon-to-amon-5} cannot be true, meaning that \pref{proof-mon-to-amon-5} is trivially satisfied. On the other hand, we know that \pref{proof-mon-to-amon-4} holds because of \pref{proof-mon-to-amon-10}. Hence, by \pref{proof-mon-to-amon-4} and \pref{proof-mon-to-amon-9} we can conclude
		\begin{gather}
				(\forall \pV\cdot \pSat \imp \monacc{\pV}{m}) \text{  and  } (\forall \pV\cdot\monacc{\pV}{m}\imp \pSat) \label{proof-mon-to-amon-11}
		\end{gather}
		By \pref{proof-mon-to-amon-11} and the defn of \textsf{pmon} we know
		\begin{gather}
			\pmondef{m}{\hV} \label{proof-mon-to-amon-12}
		\end{gather}		
	\end{case-noreset}
	\begin{case-noreset}[\pVio]
		Using a very similar argument as in the previous case, we can conclude
		\begin{gather}
			\nmondef{m}{\hV} \label{proof-mon-to-amon-13}
		\end{gather}
	\end{case-noreset}
	\noindent Hence, since $\pSat$ is the complement of $\pVio$ we can conclude that for our univerdict (sound) monitors (as shown by \pref{proof-mon-to-amon-6}), either \pref{proof-mon-to-amon-12} or \pref{proof-mon-to-amon-13} can be true but \emph{not both}. Hence, we can conclude
	\begin{gather}
		\pmondef{m}{\hV} \text{   or   }\nmondef{m}{\hV} \label{proof-mon-to-amon-14}
	\end{gather}
	By \pref{proof-mon-to-amon-14} and defn of \textsf{amon} we know
	\begin{gather*}
		\amondef{m}{\hV} 
	\end{gather*}
\end{proof}\bigskip\bigskip

\begin{proof}[ for (b)] We initially know 
	\begin{gather}
		\amondef{m}{\hV} \label{proof-amon-to-mon-1}
	\end{gather}
	By \pref{proof-amon-to-mon-1} and defn of \amondef{m}{\hV} we know 
	\begin{gather}
		\nmondef{m}{\hV} \text{  or  } \pmondef{m}{\hV} \label{proof-amon-to-mon-2}
	\end{gather}
	We individually consider the possibilities for satisfying \pref{proof-amon-to-mon-2}:
	
	\begin{case}[\text{\textsf{pmon} is \textsl{true} while \textsf{nmon} is \textsl{false}}]
		By the case hypothesis we know
		\begin{gather}
			\nmondef{m}{\hV} \text{ is \emph{true}} \label{proof-amon-to-mon-3}\\
			\pmondef{m}{\hV} \text{ is \emph{false}} \label{proof-amon-to-mon-4}
		\end{gather}
		By \pref{proof-amon-to-mon-3} and defn of \textsf{pmon} we know
		\begin{gather}
			\forall \pV\cdot\monacc{\pV}{m}\imp \pSat (\,=\,\emph{true}) \label{proof-amon-to-mon-5}\\
			\forall \pV\cdot \pSat\imp\monacc{\pV}{m} (\,=\,\emph{true}) \label{proof-amon-to-mon-6}
		\end{gather}
		By \pref{proof-amon-to-mon-4} and defn of \textsf{nmon} we know
		\begin{gather}
			\forall \pV\cdot\monrej{\pV}{m}\imp \pVio (\,=\,\emph{false}) \label{proof-amon-to-mon-7}\\
			\forall \pV\cdot \pVio\imp\monrej{\pV}{m} (\,=\,\emph{false}) \label{proof-amon-to-mon-8}
		\end{gather}
		Since \pref{proof-amon-to-mon-6} is \emph{true}, we know that $\pV\!\in\!\syn{\hV}$, however since \pref{proof-amon-to-mon-8} is \emph{false} this means that $\pV\!\notin\!\syn{\hV}$ as otherwise the entire implication (\ie \pref{proof-amon-to-mon-8}) would resolve to \emph{true}. Hence, this case is satisfied trivially since \pref{proof-amon-to-mon-6} and \pref{proof-amon-to-mon-8} \emph{contradict} each other.		
	\end{case}
	
	\begin{case}[\text{\textsf{pmon} is \textsl{false} while \textsf{nmon} is \textsl{true}}] The proof for this case is very similar to that for the other cases.
	\end{case}
	
	\begin{case}[\text{Both \textsf{pmon} and \textsf{nmon} are \textsl{true}}]
		By the case hypothesis we know
		\begin{gather}
			\nmondef{m}{\hV} \text{ is \emph{true}} \label{proof-amon-to-mon-9}\\
			\pmondef{m}{\hV} \text{ is \emph{true}} \label{proof-amon-to-mon-10}
		\end{gather}
		By \pref{proof-amon-to-mon-9} and defn of \textsf{pmon} we know
		\begin{gather}
			\forall \pV\cdot\monacc{\pV}{m}\imp \pSat (\,=\,\emph{true}) \label{proof-amon-to-mon-11}\\
			\forall \pV\cdot \pSat\imp\monacc{\pV}{m} (\,=\,\emph{true}) \label{proof-amon-to-mon-12}
		\end{gather}
		By \pref{proof-amon-to-mon-10} and defn of \textsf{nmon} we know
		\begin{gather}
			\forall \pV\cdot\monrej{\pV}{m}\imp \pVio (\,=\,\emph{true}) \label{proof-amon-to-mon-13}\\
			\forall \pV\cdot \pVio\imp\monrej{\pV}{m} (\,=\,\emph{true}) \label{proof-amon-to-mon-14}
		\end{gather}
		Hence, by \pref{proof-amon-to-mon-11}, \pref{proof-amon-to-mon-13} and defn of \textsf{smon} we know
		\begin{gather}
			\smondef{m}{\hV} \label{proof-amon-to-mon-15}
		\end{gather}
		By introducing a disjunction on \pref{proof-amon-to-mon-12} and \pref{proof-amon-to-mon-14}, we know
		\begin{gather}
			(\pSat \imp \monacc{\pV}{m}) \text{  or  } (\pVio \imp \monrej{\pV}{m}) \label{proof-amon-to-mon-16}
		\end{gather}
		By \pref{proof-amon-to-mon-16} and defn of \textsf{cmon} we know
		\begin{gather}
			\cmondef{m}{\hV} \label{proof-amon-to-mon-17}
		\end{gather}
		By \pref{proof-amon-to-mon-15}, \pref{proof-amon-to-mon-17} and defn of \textsf{mon} we know
		\begin{gather}
			\mondef{m}{\hV} \label{proof-amon-to-mon-18}
		\end{gather}
	\end{case}	
\end{proof}
