# Supplementary material for: Developing Theoretical Foundations for Runtime Enforcement
Source: arXiv:1804.08917 source file (2018-11-12)
Supplement: Supplementary file 3 [file rel-mon-enf-proof.tex]

\begin{rtp}
	$\forall\hV\in\uhml\cdot\, \enfmonrel{\g{\hV}{\rho}}{\gRV{\hV}}$\\[2mm]
	To Prove this theorem we must show that relation \R (below) \emphbf{relates enforceability to monitorability}.
	$$\R \defEquals \big\{(\g{\hV}{\rho},\gRV{\hV})\;\vert\; \g{\hV}{\rho}=\eV \text{ and }\gRV{\hV}=\mV \big\}$$
\end{rtp}

\ic{I'M NOT ENTIRELY SURE WHETHER THIS PROOF MAKES ANY SENSE!!!!}

\begin{proof} By coinduction on the structure of $\hV$. 
	\\\begin{proofRemark}
		[Since \g{\hV} is defined exclusively for formulae that are expressible in \shmlwf, any other formula $\hV\in\uhml$ but $\hV\notin\shmlwf$ cannot be synthesised into an enforcement monitor and thus cause the premise of the theorem being proven to evaluate to false, thereby leading the theorem to be trivially satisfied. Hence, it suffices to conduct our coinductive proof \wrt $\hV\in\shmlwf$.\medskip]
	\end{proofRemark}\vspace{-5mm}

	\begin{case}[\hV=\htru] \ic{THIS CASE IS CAUSING TROUBLE!!}	\end{case} 
	
	\begin{case}[\hV=\hVarX] Does not apply since $\hVarX$ is an open formula. \end{case} 	

	\begin{case}[\hV=\hfls] 
		\newcommand{\formula}{\hfls}
		Initially we know
		\begin{gather}
			\enfdef{\g{\formula}{\rho}}{\formula}\label{proof:enf-mon-rel-ff-1}
		\end{gather}
		Since $\hV=\formula$, by defn of \g{-} and \gRV{-} we know
		\begin{gather}
			\g{\formula}{\rho}=\mend \label{proof:enf-mon-rel-ff-2}\\
			\gRV{\formula}=\mno \label{proof:enf-mon-rel-ff-3}
		\end{gather}
		Since \formula cannot be satisfied by any process $\pV$, we can deduce
		\begin{gather}
			\forall \pV\cdot\, \pV\nvSat\formula \label{proof:enf-mon-rel-ff-4}
		\end{gather}
		Moreover, from \pref{proof:enf-mon-rel-ff-3} and the defn of \textsf{rej}, we know
		\begin{gather}
			\forall \pV\cdot\, \monrej{\pV}{\gRV{\formula}} \label{proof:enf-mon-rel-ff-5}
		\end{gather}
		By \pref{proof:enf-mon-rel-ff-4} and \pref{proof:enf-mon-rel-ff-5}, we can thus deduce
		\begin{gather}
			\forall \pV\cdot\, \pV\nvSat\formula\, \imp\, \monrej{\pV}{\gRV{\formula}} \label{proof:enf-mon-rel-ff-6}\\
			\forall \pV\cdot\, \monrej{\pV}{\gRV{\formula}}\, \imp\, \pV\nvSat\formula \label{proof:enf-mon-rel-ff-7}
		\end{gather}
		Finally, by \pref{proof:enf-mon-rel-ff-6}, \pref{proof:enf-mon-rel-ff-7} and the defn of \textsf{nmon} we know
		\begin{gather}
			\nmondef{\gRV{\formula}}{\formula}
		\end{gather}
	\end{case} 
		
	\begin{case}[\hV=\hmax{\hVarX}{\hV}]
		\newcommand{\formula}{\hmax{\hVarX}{\hV}}
		\newcommand{\subform}{\hV\sub{\formula}{\hVarX}}
		\newcommand{\recsubenf}{\g{\hV}{\rho}\sub{\mrec{\mx}{\g{\hV}{\rho}}}{\mx}}
		\newcommand{\recsubmon}{\gRV{\hV}{\rho}\sub{\mrec{\mx}{\gRV{\hV}{\rho}}}{\mx}}
		Initially we know
		\begin{gather}
			\enfdef{\g{\formula}{\rho}}{\formula}\label{proof:enf-mon-rel-max-1}
		\end{gather}
		Since $\formula\,\equiv\,\subform$, from \pref{proof:enf-mon-rel-max-1} we know
		\begin{gather}
			\enfdef{\g{\subform}{\rho}}{\subform}\label{proof:enf-mon-rel-max-2}
		\end{gather}
		Since $\hV=\formula$, by defn of \g{-} and \gRV{-} we know
		\begin{gather}
			\g{\formula}{\rho}=\recsubenf \label{proof:enf-mon-rel-max-3}\\
			\gRV{\formula}=\recsubmon \label{proof:enf-mon-rel-max-4}
		\end{gather}
		By \pref{proof:enf-mon-rel-max-3}, \pref{proof:enf-mon-rel-max-4} and defn of \R we know
		\begin{gather}
			(\recsubenf,\recsubmon)\in\R \label{proof:enf-mon-rel-max-5}
		\end{gather}
		By \pref{proof:enf-mon-rel-max-5} and IH we know
		\begin{gather}
			\enfdef{\recsubenf}{\subform} \imp \nmondef{\recsubmon}{\subform} \label{proof:enf-mon-rel-max-6}
		\end{gather}
		By \pref{proof:enf-mon-rel-max-3}, \pref{proof:enf-mon-rel-max-6} and since $\formula\,\equiv\,\subform$ we know
		\begin{gather}
			\enfdef{\g{\formula}{\rho}}{\formula} \imp \nmondef{\recsubmon}{\subform} \label{proof:enf-mon-rel-max-7}
		\end{gather}
		From \pref{proof:enf-mon-rel-max-1} and \pref{proof:enf-mon-rel-max-7} we deduce
		\begin{gather}
			\nmondef{\recsubmon}{\subform} \label{proof:enf-mon-rel-max-8}
		\end{gather}
		Finally, by \pref{proof:enf-mon-rel-max-3}, \pref{proof:enf-mon-rel-max-4}, \pref{proof:enf-mon-rel-max-8} and since $\formula\,\equiv\,\subform$ we conclude
		\begin{gather}
			\nmondef{\gRV{\formula}}{\formula}
		\end{gather}		
	\end{case} 	

	\begin{case}[\hV=\hAnd\hgnec{\pate_i}{c_i}\hV_i]
		\newcommand{\formula}{\hAnd\hgnec{\pate_i}{c_i}\hV_i}
		\newcommand{\subenf}{
			\begin{xbrackets}{c}
			\mCh
			\begin{xbrace}{ll}
				\mdropc{\pate_i}{c_i}{\g{\varphi_i}{\rho}} & \quad \text{if }\dc{{\varphi_i}}=\ctru\!\!\!\\
				\mact{\pate_i}{c_i}{\g{\varphi_i}{\rho}} & \quad \text{otherwise} \!\!\!
			\end{xbrace}
			\end{xbrackets}}
		\newcommand{\submon}{\mCh\mact{\pate_i}{c_i}{\gRV{\varphi_i}}}
		Initially we know
		\begin{gather}
		\enfdef{\g{\formula}{\rho}}{\formula}\label{proof:enf-mon-rel-nec-1}
		\end{gather}
		Since $\hV=\formula$, by defn of $\g{-}{\rho}$ and \gRV{-} we know
		\begin{gather}
			\g{\formula}{\rho}=\subenf \label{proof:enf-mon-rel-nec-2}\\
			\gRV{\formula}=\mCh\gRV{\hgnec{\pate_i}{c_i}{\varphi_i}}=\submon \label{proof:enf-mon-rel-nec-3}
		\end{gather}
		By \pref{proof:enf-mon-rel-nec-2}, \pref{proof:enf-mon-rel-nec-3} and defn of \R we know
		\begin{gather}
			(\subenf,\submon)\in\R \label{proof:enf-mon-rel-nec-4}
		\end{gather}
		By \pref{proof:enf-mon-rel-nec-4} and IH we know
		\begin{gather}
			\begin{array}{r}
				\enfdef{\subenf}{\formula} \\ \hfill\imp \nmondef{\submon}{\formula} 
			\end{array}\label{proof:enf-mon-rel-nec-5}
		\end{gather}
		From \pref{proof:enf-mon-rel-nec-1}, \pref{proof:enf-mon-rel-nec-2} and \pref{proof:enf-mon-rel-nec-5} we can deduce
		\begin{gather}
			\nmondef{\submon}{\formula} \label{proof:enf-mon-rel-nec-6}
		\end{gather}
		Finally, by \pref{proof:enf-mon-rel-nec-5} and \pref{proof:enf-mon-rel-max-6} we can conclude
		\begin{gather}
			\nmondef{\gRV{\formula}}{\formula}
		\end{gather}		
	\end{case}	
\end{proof}
